# Supplementary material for: No-Regret Caching via Online Mirror Descent
Source: arXiv:2101.12588 source file (2023-06-06)
Supplement: Supplementary file 3 [file Z-CacheNetworks-Appendix.tex]

% \NewAppendix{Network of Caches Proofs}
\clearpage
\begin{center}
{\Large  Caching Networks: Proofs}
\end{center}

\section{Sufficiency of First Moment State Representation}
\begin{proposition}
\label{p:cn_moments}
Any random  independent cache states  $\z^v_t \in \statesSetInt^v$ with expected value $\mathbb{E}[\z^v_t] = \x^v_t$, where $\x^v_t \in \statesSetFrac^v$, incur the same expected gain as the random cache states $\bar\z^v_t$ constructed using  Algorithm~\ref{algo:online_coupled_rounding} with input $\x_t^v$ and $\xi^v$ drawn independently for each cache nodes $v \in \vertices$.
\end{proposition}
\begin{proof}
\begin{align}
    \mathbb{E} \left[G_{\vec r_t}( \z_t)\right] &=  \mathbb{E} \left[      \sum_{(i,\vec\path) \in \requestSet} r_{t, (i, \vec \path)} \sum^{|\vec\path|-1}_{k=1} \weight_{\left(\path_k,\path_{k+1}\right)} \min\left\{1, \sum^k_{k'=1} z^{\path_{i'}}_{i'}\right\}\right]\\
    &= \mathbb{E} \left[ \sum_{(i,\vec\path) \in \requestSet} r_{t, (i, \vec \path)} \sum^{|\vec\path|-1}_{k=1} \weight_{\left(\path_k,\path_{k+1}\right)} \left(1 - \prod^k_{k'=1} (1-  z^{p_{k'}}_{i})\right)\right] \\
    &= \label{e:cn_linearity_of_expectation} \sum_{(i,\vec\path) \in \requestSet} r_{t, (i, \vec \path)} \sum^{|\vec\path|-1}_{k=1} \weight_{\left(\path_k,\path_{k+1}\right)} \left(1 - \mathbb{E} \left[\prod^k_{k'=1} (1-  z^{p_{k'}}_{i})\right]\right)\\
    &=  \label{e:cn_independence} \sum_{(i,\vec\path) \in \requestSet} r_{t, (i, \vec \path)} \sum^{|\vec\path|-1}_{k=1} \weight_{\left(\path_k,\path_{k+1}\right)} \left(1 - \prod^k_{k'=1} (1-  x^{p_{k'}}_{i})\right).
\end{align}
Eq.~\eqref{e:cn_linearity_of_expectation} is obtained using linearity of expectation and Eq.~\eqref{e:cn_independence} is obtained since $\z^v$ and $\z^{v'}$ are independent for   $v \neq v'$ and $v, v' \in \vertices$. Algorithm~\ref{algo:online_coupled_rounding} is called on fractional cache state $\x^v_t$ and $\xi^v$, then the obtained random cache state $\bar\z^v_t$ is independent with $\bar\z^{v'}_t$ for $v \neq v'$ and $\mathbb{E}\left[\z'^v_t\right] = \x^v_t$ for every $v', v \in \vertices$; therefore,  the random cache states  $\z^v_t$ have the same expected gain as the random cache states $\bar \z^v_t$, i.e., 
\begin{align}
    \mathbb{E} \left[G_{\vec r_t}( \bar\z_t)\right]   = \mathbb{E} \left[G_{\vec r_t}( \z_t)\right].
\end{align}

\end{proof}
\section{Subgradient Expression}
\label{appendix:subgradient_expression}
\begin{lemma}
The gain function in Eq.~\eqref{e:gain_cache_network} has a subgradient $\vec g_t$ at point $\x_t \in \statesSetFrac$ given by
\begin{align}
    \vec g_t = \left[\sum_{(i,\vec\path) \in \requestSet_i}  r_{t, (i, \vec \path)} \sum^{|\vec\path|-1}_{k=k_{\vec \path} (v)}  \weight_{\left(\path_k,\path_{k+1}\right)} \mathds{1}_{\left\{\sum^k_{k'=1}x^{\path_{k'}}_{i} <  1 \right\}}\right]_{(v,i) \in \vertices \times \catalog}
\end{align}
\end {lemma}
\begin{proof}
The function given by $ \x \to \min\left\{1, \sum^k_{k'=1} x^{\path_{k'}}_{i}\right\}$ is a minimum of two concave differentiable functions (a constant, and an affine function). We can characterize its subdifferential (set of all possible subgradients), using \cite[Theorem 8.2]{mordukhovich2017geometric}, at point $\x_t \in \statesSetFrac$ as
   \begin{align}
       \partial \left(\min\left\{1, \sum^k_{k'=1} x^{\path_{k'}}_{i}\right\} \right)= \begin{cases}
      \left\{ \nabla ( \sum^k_{k'=1}x^{\path_{k'}}_{i})\right\} &\mathrm{if}\,\,\sum^k_{k'=1} x^{\path_{k'}}_{i} < 1, \\
      \conv{\left\{\vec{0}, \nabla ( \sum^k_{k'=1}x^{\path_{k'}}_{i})\right\}} &\mathrm{if}\,\,\sum^k_{k'=1} x^{\path_{k'}}_{i} = 1 , \\
      \{\vec{0}\}  &\mathrm{otherwise}\
     ,
       \end{cases}
   \end{align}
where $\conv{\,\cdot\,}$ is the convex hull of a set, and the gradient $\nabla$ is given by $\nabla (\,\cdot\,) = [\frac{\partial\phantom{x^v_i}}{\partial x^v_i} (\,\cdot\,)]_{(v,i) \in \vertices \times \catalog}$. The operator $\frac{\partial\phantom{x^v_i}}{\partial x^v_i} (\,\cdot\,)$ is the partial derivative w.r.t $x^v_i$ (not to be confused with the subdifferential notation). 

We can restrict ourselves to the valid subgradient $\tilde{\vec{g}}^k_{(i, \vec\path),t} \in \partial \left(\min\left\{1, \sum^k_{k'=1} x^{\path_{k'}}_{i}\right\} \right)$ given by
\begin{align}
    \tilde{\vec{g}}^k_{(i, \vec\path),t} \triangleq \begin{cases}
       \nabla \left(\sum^k_{k'=1}x^{\path_{k'}}_{i}\right) & \mathrm{if}\,\, \sum^k_{k'=1}x^{\path_{k'}}_{i} <  1, \\
     \vec{0} , & \mathrm{otherwise}.
       \end{cases}
       \label{eq:subgradient_instance}
\end{align}
Note that for any $(v,i') \in \vertices \times \catalog$ and $(i,\vec\path)\in \requestSet$ we have
\begin{align}
    \deriv{\sum^k_{k'=1}x^{\path_{k'}}_{i} }{x^v_{i'}} = \sum^k_{k'=1} \deriv{x^{\path_{k'}}_{i}}{x^v_{i'}}  = \mathds{1}_{\{ i = i' \land k_{\vec \path} (v) \leq k  \}}.
\end{align}
Since there are no repeating nodes in a simple path, then the partial derivative w.r.t $x^v_i$ is non-zero only if $v$ is among the nodes $k$-hops away from the request source along the path $\vec \path$ and the file requested is $i$, i.e., the condition $i = i' \land k_{\vec \path} (v) \leq k$. We can reformulate Eq.~\eqref{eq:subgradient_instance} as 
\begin{align}
\tilde{{g}}^{k,v}_{(i, \vec\path),t, i'} &\triangleq \begin{cases}
       \mathds{1}_{\{ i = i' \land k_{\vec \path} (v) \leq k  \}} & \mathrm{if}\,\, \sum^k_{k'=1}x^{\path_{k'}}_{i} <  1, \\
     0 , & \mathrm{otherwise}.
       \end{cases} = \mathds{1}_{\left\{i = i' \land k_{\vec \path} (v) \leq k \land \sum^k_{k'=1}x^{\path_{k'}}_{i} <  1 \right\} }.
\end{align}
By considering the subdifferential
\begin{align}
    \partial G_{\vec r_t} (\x_t) = \partial \left( \sum_{(i,\vec\path) \in \requestSet}  \sum^{|\vec\path|-1}_{k=1} r_{t, (i, \vec \path)} \weight_{\left(\path_k,\path_{k+1}\right)} \min\left\{1, \sum^k_{k'=1} x^{\path_{k'}}_{i}\right\}\right),
\end{align}
and using \cite[Theorem 23.6]{rockafellar2015convex}, we get 
\begin{align}
    \partial G_{\vec r_t} (\x_t) = \sum_{(i,\vec\path) \in \requestSet} \sum^{|\vec\path|-1}_{k=1}  \partial \left(r_{t, (i, \vec \path)} \weight_{\left(\path_k,\path_{k+1}\right)}  \min\left\{1, \sum^k_{k'=1} x^{\path_{k'}}_{i}\right\}\right),
\end{align}
The constant factors $ r_{t, (i, \vec \path)} $ and $\weight_{\left(\path_k,\path_{k+1}\right)}$ are non-negative, so we can multiply both sides of the subgradient inequality by a non-negative constant \cite[Sec.~23]{rockafellar2015convex}. We get 
\begin{align}
    \partial G_{\vec r_t} (\x_t) = \sum_{(i,\vec\path) \in \requestSet}  r_{t, (i, \vec \path)} \sum^{|\vec\path|-1}_{k=1}  \weight_{\left(\path_k,\path_{k+1}\right)} \partial \left( \min\left\{1, \sum^k_{k'=1} x^{\path_{k'}}_{i}\right\}\right).
\end{align}
Then, a subgradient $\vec{g}_t \in \partial G_{\vec r_t} (\x_t)$ at point $\x_t \in \statesSetFrac$ is given by
\begin{align}
    \vec g_t = \sum_{(i,\vec\path) \in \requestSet}  r_{t, (i, \vec \path)} \sum^{|\vec\path|-1}_{k=1}  \weight_{\left(\path_k,\path_{k+1}\right)} \tilde{\vec{g}}^k_{(i, \vec\path),t}.
\end{align}
The $(v,i)$-th component of such subgradient is 
\begin{align}
    g^v_{t,i} &= \sum_{(i',\vec\path) \in \requestSet}  r_{t, (i', \vec \path)} \sum^{|\vec\path|-1}_{k=1}  \weight_{\left(\path_k,\path_{k+1}\right)} \tilde{{g}}^{k,v}_{(i', \vec\path),t, i} =   \sum_{(i',\vec\path) \in \requestSet}  r_{t, (i', \vec \path)} \sum^{|\vec\path|-1}_{k=1}  \weight_{\left(\path_k,\path_{k+1}\right)} \mathds{1}_{\left\{i = i' \land k_{\vec \path} (v) \leq k \land \sum^k_{k'=1}x^{\path_{k'}}_{i'} <  1 \right\} } \\
    &=  \sum_{(i,\vec\path) \in \requestSet_i}  r_{t, (i, \vec \path)} \sum^{|\vec\path|-1}_{k=1}  \weight_{\left(\path_k,\path_{k+1}\right)} \mathds{1}_{\left\{k_{\vec \path} (v) \leq k \land \sum^k_{k'=1}x^{\path_{k'}}_{i} <  1 \right\} } = \sum_{(i,\vec\path) \in \requestSet_i}  r_{t, (i, \vec \path)} \sum^{|\vec\path|-1}_{k=k_{\vec \path} (v)}  \weight_{\left(\path_k,\path_{k+1}\right)} \mathds{1}_{\left\{\sum^k_{k'=1}x^{\path_{k'}}_{i} <  1 \right\} }.
\end{align}
This concludes the proof.
\end{proof}
\section{Supporting Lemmas for the Proof of Theorem~\ref{theorem:cn_regret_fractional}}
\subsection{The Global Mirror Map Equivalently Describes the Evolution of the Cache States}
\begin{lemma}
\label{lemma:cn_global_mirror_map}
The collection of OMA policies running \LocalAlgoName{} in Algorithm~\ref{algo:cn_online_mirror_ascent} at each node $v \in \vertices$ is equivalent to running OMA configured with the global mirror map $\Phi: \domainPhi \to \mathbb{R}$ given by
\begin{align}
    \Phi(\x) = \sum_{v \in \vertices} \Phi^v(\x),
\end{align}
where $\Phi^v: \domainPhi^v \to \mathbb{R}$ is the local mirror map of node $v \in \vertices$.
\end{lemma}
\begin{proof}
Let $\x^v_1 \in \statesSetFrac^v$ be the intitial value at each node $v\in \vertices$. Using Lemma~\ref{lemma:condition_on_states}, the states $\x_{t+1}$ satisfy the following for any $t \in [T]$ 
\begin{align}
       (\nabla \Phi^v(\x^v_{t+1})-\nabla \Phi^v(\x^v_t) - \eta \vec g^v_t )^T (\x^v_{t+1} - \x^v)    &\leq 0, \forall \x^v \in \statesSetFrac^v \cap \domainPhi^v.
\end{align}
We obtain from the previous Eq. the following
 \begin{align}
      \sum_{v \in \vertices} (\nabla \Phi^v(\x^v_{t+1})-\nabla \Phi^v(\x^v_t) - \eta \vec g^v)^T (\x^v_{t+1} - \x^v) &= \left(\sum_{v \in \vertices}\left(\nabla \Phi^v(\x^v_{t+1})-\nabla \Phi^v(\x^v_t) - \eta \vec g^v\right)  \right)^T \left(\sum_{v \in \vertices} {\x^v_{t+1} - \x^v}\right)\\
      &= \left(\nabla \Phi(\x^v_{t+1})-\nabla \Phi(\x^v_t) - \eta \vec g_t\right)^T (\x_{t+1}- \x) \leq 0,\\
      &\forall \x \in \statesSetFrac \cap \domainPhi.
 \end{align}
 
 Therefore, the augmented state $\x_{t+1} = \sum_{v \in \vertices}\x^v_{t+1}$ from each local node $v\in\vertices$ corresponds to states obtained by OMA configured by the global mirror map $\Phi$ when initialized by $\x_{1} = \sum_{v \in \vertices}\x^v_{1}$ for every $t \in [T]$.
\end{proof}
\subsection{Concavity of the Gain Function}
\begin{lemma}
The gain function given by Eq.~\eqref{e:gain_cache_network} is concave over its domain $\statesSetFrac$ of possible fractional cache states.
\label{lemma:concavity}
\end{lemma}
\begin{proof}
For any $\vec r \in \setRequestBatch$, $(i,\vec \path) \in \requestSet$, and $k \in [|\vec\path|-1]$, the factors $r_{(i,\vec \path)} w_{(\path_{k}, \path_{k+1})}$ are non-negative. The function $\x\to \min\left\{1, \sum^k_{k'=1} x^{\path_{k'}}_{i}\right\}$ is the minimum between a constant $1$ and a sum  $\sum^{k}_{k'=1} x^{\path_{k'}}_{i}$ of linear functions of $\x$. Such minimum is thus a concave function of $\x$. Therefore, the gain in Eq.~\eqref{e:gain_cache_network} is a weighted sum with non-negative weights of concave functions in $\x$, which is concave. 
\end{proof}


\begin{lemma}
Let $\x^v \in \statesSetFrac^v$ be a fractional cache state of node $v$, and $\z^v \in \statesSetInt^v$ be a random cache state of node $v$ such that: 
\begin{enumerate}
    \item $\mathbb{E}[\z^v] = \x^v, \forall v \in \vertices$,
    \item  and $\z^u$ is independent with $\z^{v}$ for any $(u,v) \in \vertices^2 $ and $u \neq v$.
\end{enumerate}
We get that the expected gain at state $\z = \sum_{v \in \vertices} \z^v$ is at least $1-\frac{1}{e}$ of the gain evaluated at the fractional state $\x = \sum_{v\in \vertices} \x^v$, i.e., 
\begin{align}
    \mathbb{E} [G_{\vec r} (\z)] \geq  \left(1-\frac{1}{e}\right)G_{\vec r} (\x), \forall \vec r \in \setRequestBatch.
    \label{eq:cn_lower_bound}
\end{align}
\end{lemma}
\begin{proof}

We define the following surrogate function for any $\vec r \in \setRequestBatch$ that we use to bound the gain function
\begin{align}
    \Lambda_{\vec r} (\x) = \sum_{(i,\vec\path) \in \requestSet} r_{t, (i, \vec \path)} \sum^{|\vec\path|-1}_{k=1} \weight_{\left(\path_k,\path_{k+1}\right)} \left(1 - \prod^k_{k'=1} x^{\path_{k'}}_{i}\right).
\end{align}
% We have 
% \begin{align}
%     \mathbb{E} [G_{\vec r} (\z)]  &=  \mathbb{E} \left[  \sum_{(i,\vec\path) \in \requestSet} r_{t, (i, \vec \path)} \sum^{|\vec\path|-1}_{k=1} \weight_{\left(\path_k,\path_{k+1}\right)} \min\left\{1, \sum^k_{k'=1} z^{\path_{k'}}_{i}\right\} \right]  =   \sum_{(i,\vec\path) \in \requestSet} r_{t, (i, \vec \path)} \sum^{|\vec\path|-1}_{k=1} \weight_{\left(\path_k,\path_{k+1}\right)} \mathbb{E} \left[ \min\left\{1, \sum^k_{k'=1} z^{\path_{k'}}_{i}\right\} \right]\\
%     & \leq \sum_{(i,\vec\path) \in \requestSet} r_{t, (i, \vec \path)} \sum^{|\vec\path|-1}_{k=1} \weight_{\left(\path_k,\path_{k+1}\right)} \min\left\{1, \sum^k_{k'=1} x^{\path_{k'}}_{i}\right\} = G_{\vec r} (\x).
%     \label{eq:bounding_gain_upper}
% \end{align}
% The inequality is obtained using Jensen's inequality and the concavity of $\x\to\min\left\{1, \sum^k_{k'=1} x^{\path_{k'}}_{i}\right\}$ for any $(i, \vec\path) \in \requestSet$, $k \in [|\vec \path|-1]$, and $\x \in \statesSetFrac$. 
The surrogate function evaluated at a fractional cache network state $\x$ is equal of the expected gain of random cache network state $\z$. We have the following
\begin{align}
     \mathbb{E} [G_{\vec r} (\z)]  &=  \mathbb{E} \left[  \sum_{(i,\vec\path) \in \requestSet} r_{t, (i, \vec \path)} \sum^{|\vec\path|-1}_{k=1} \weight_{\left(\path_k,\path_{k+1}\right)} \min\left\{1, \sum^k_{k'=1} z^{\path_{k'}}_{i}\right\} \right]\\
     &= \mathbb{E} \left[  \sum_{(i,\vec\path) \in \requestSet} r_{t, (i, \vec \path)} \sum^{|\vec\path|-1}_{k=1} \weight_{\left(\path_k,\path_{k+1}\right)} \left(1 - \prod^k_{k'=1} (1-z^{\path_{k'}}_{i})\right) \right] \\
     &= \Lambda_{\vec r}(\x).  
     \label{eq:bounding_gain_equal}
\end{align}
The last equality is obtained using the linearity of expectations and the independence of the random variables $\z^v$ and $z^{v'}$ for all $v,v' \in \vertices$ and $v\neq v'$.
% We combine Eq.~\eqref{eq:bounding_gain_upper} and Eq.~\eqref{eq:bounding_gain_equal} to get 
% \begin{align}
%     \Lambda_{\vec r}(\x) \leq G_{\vec r} (\x).
% \end{align}

Goemans and Williamson~\cite[Lemma 3.1]{goemans1994new} proved for any $x_k' \in [0,1], \forall k'\in[k]$ (take $z_j = \min\{1, \sum^k_{k'=1} x_{k'}\}$) the following inequality 
\begin{align}
\left(1 - \prod^k_{k'=1} (1-x^{\path_{k'}}_{i})\right) \geq \left(1-\frac{1}{e}\right) \min\left\{1, \sum^k_{k'=1} x^{\path_{k'}}_{i}\right\}.
\label{eq:sat_inequality}
\end{align}
We can use the above inequality to obtain the lower bound
\begin{align}
    \Lambda_{\vec r}(\x) &= \sum_{(i,\vec\path) \in \requestSet} r_{t, (i, \vec \path)} \sum^{|\vec\path|-1}_{k=1} \weight_{\left(\path_k,\path_{k+1}\right)} \left(1 - \prod^k_{k'=1} (1-x^{\path_{k'}}_{i})\right)\\
    &\stackrel{\eqref{eq:sat_inequality}}{\geq} \left(1 - \frac{1}{e}\right) \sum_{(i,\vec\path) \in \requestSet} r_{t, (i, \vec \path)} \sum^{|\vec\path|-1}_{k=1} \weight_{\left(\path_k,\path_{k+1}\right)} \min\left\{1, \sum^k_{k'=1} x^{\path_{k'}}_{i}\right\}
    = \left(1 - \frac{1}{e}\right)G_{\vec r_t} (\x).
\end{align}

We conclude that 
\begin{align}
     \mathbb{E}[G_{\vec r}(\z)] \geq \left(1 - \frac{1}{e}\right)G_{\vec r_t} (\x), \forall \vec r \in \setRequestBatch.
\end{align}
\end{proof}
\section{Proof of Theorem~\ref{theorem:cn_regret_fractional}}
\label{proof:cn_regret_fractional}
\begin{proof}
Fix a sequence of request batches $\{\vec r_t\}^T_{t=1}$, and a fractional caching network state $\x \in\statesSetFrac$. From Lemma~\ref{lemma:concavity}, the gain function $G_{\vec r_t}$ is concave over the fractional domain $\statesSetFrac$ we obtain
\begin{align}
   \sum^T_{t=1} G_{\vec r_t} (\x) - G_{\vec r_t} (\x_t) &\leq\sum^T_{t=1} \vec g_t^T (\x - \x_t)  = \sum_{v \in \vertices} \left(\vec g^v_t\right)^T (\x^v - \x^v_t).
   \label{eq:cn_concavity_expand}
\end{align}
Using Lemma~\ref{lemma:cn_global_mirror_map}, Eq.~\eqref{eq:cn_concavity_expand}, and lines 6--8 in Algorithm~\ref{algo:cn_online_mirror_ascent} we obtain the following 
\begin{align}
     \sum^T_{t=1} G_{\vec r_t} (\x) - G_{\vec r_t} (\x_t) = \sum^T_{t=1}\sum_{v \in \vertices} \frac{1}{\eta^v} \left(\nabla \Phi^v(\x_t^v) - \Phi^v(\y_{t+1}^v)\right) (\x^v_t - \x^v ),
\end{align}
and following the proof of Theorem~4.2 in \cite{bubeck2015convexbook} we obtain
 \begin{align}
  &\sum^T_{t=1} G_{\vec r_t} (\x) - G_{\vec r_t} (\x_t)\\&\leq 
     \sum^T_{t=1} \sum_{v \in \vertices} \frac{1}{\eta^v} \left( \vGroup{D_{\Phi^v}(\x^v,\x^v_t )- D_{\Phi^v}(\x^v,\x^v_{t+1})}{\text{telescoping term}}  + \vGroup{D_{\Phi^v}(\x^v_t, \y^v_{t+1}) - D_{\Phi^v}(\x^v_{t+1}, \y^v_{t+1})}{\leq (\eta^v L^v_{\max})^2/(2\theta^v)}\right)^T(\x^v_t - \x^v )\\
    &\leq \sum_{v \in \vertices} \left(\frac{ D_{\Phi^v}(\x^v,\x^v_1 )}{\eta^v} + \frac{\eta^v \left(L^v_{\max}\right)^2}{ 2 \theta^v} T \right) \leq  \sum_{v \in \vertices}  \left(\frac{D^v_{\max}}{\eta^v} + \frac{\eta^v \left(L^v_{\max}\right)^2}{ 2 \theta^v} T \right).\label{eq:cn_raw_regret}
\end{align}
\end{proof}
By taking the limit $\x\to \x_*$, and the above upper bound holds for an arbitrary sequence of request batches $\{\vec r_t\}^T_{t=1}$; therefore, the regret is given as 
\begin{align}
     \text{Regret}_{T, \statesSetFrac}(\text{OMA}_{\Phi^{\vertices}}) &=\underset{
{{\{\vec r_t \}_{t=1}^{T} \in \setRequestBatch^T}}
}{\sup}   \left\{ \sum^T_{t=1}    G_{\vec r_t}( \x_*){-}\sum^T_{t=1}    G_{\vec r_t}(\x_t) \right\} \leq  \sum_{v \in \vertices}  \left(\frac{D^v_{\max}}{\eta^v} + \frac{\eta^v \left(L^v_{\max}\right)^2}{ 2 \theta^v} T \right) ,
\end{align}
and selecting for every node $v \in \vertices$ the learning rates  $\eta^v = \frac{1}{L^v_{\max}} \sqrt{\frac{2 \theta^v D^v_{\max}}{T}}$ giving the tightest regret bound we finally obtain 
\begin{align}
     \text{Regret}_{T, \statesSetFrac}(\text{OMA}_{\Phi^{\vertices}}) \leq \left(\sum_{v \in \vertices} L^v_{\max} \sqrt{\frac{2 D^v_{\max}}{\theta^v} }\right) \sqrt{T}.
\end{align}
\section{Proof of Theorem~\ref{theorem:cn_fractional_offline_problem}}
\label{proof:cn_fractional_offline_problem}
\begin{proof}
Let $\bar \x$ be the average fractional caching network state $\bar \x = \frac{1}{K} \sum^K_{k=1} \x_k $, and  $\vec g_k$ be the sub-gradient of the fixed gain function in~\eqref{eq:cn_static_gain_fractional} obtained at iteration $k$, and $G_T$ is the average of concave functions (see Lemma~\ref{lemma:concavity}), then $G_T$ is also concave and  we have from Jensen's inequality 
\begin{align}
G_T(\bar\x)\geq \frac{1}{K}\sum^K_{k=1} G_T(\x_k), 
\end{align}
and
\begin{align}
 G_T(\x) - G_T(\bar\x) \leq  \frac{1}{K}  \left( \sum^K_{k=1} G_T(\x) - \sum^K_{t=1} G_T(\x_k)\right) \leq\frac{1}{K} \vec g^T (\x - \x_k).  
\end{align}

Observe that the bound in Eq.~\eqref{eq:cn_raw_regret} is obtained obliviously whether the subgradients are drawn from a  time-variant function or a fixed function, so if we select $\eta^v = \frac{1}{L^v_{\max}} \sqrt{\frac{2 \theta^v D^v_{\max}}{K}}$ for every $v \in\vertices$ we get
\begin{align}
  G_T(\x) - G_T(\bar\x)  \leq \left(\sum_{v \in \vertices} L^v_{\max} \sqrt{\frac{2 D^v_{\max}}{\theta^v} }\right) \frac{1}{\sqrt{K}}.
\end{align} 
With a rearrangement we get 

\begin{align}
    G_T(\bar\x)   \geq  G_T(\x)  - \left(\sum_{v \in \vertices} L^v_{\max} \sqrt{\frac{2 D^v_{\max}}{\theta^v} }\right) \frac{1}{\sqrt{K}}.
    \label{eq:cn_static_ineq}
\end{align}

Taking the limit $\x \to \x_*$ concludes the proof.


\end{proof}
\section{Some Properties of Neg-Entropy and Euclidean Mirror Maps }
\label{appendix:cn_properties_mp}
When $\Phi$ is the Euclidean mirror map, assumption (A1)--(A2) in Sec.~\ref{sec:cn_regret_analysis} are satisfied as follows: 
\begin{enumerate}
    \item $\Phi$ is a mirror map (see Sec.~\ref{section:OMD}).
    \item  $\Phi$ is $\theta^v$-strongly convex w.r.t $\norm{\,\cdot\,}_2 = d^v({\,\cdot\,}) $, where $\theta^v=1$ (see \cite[Lemma 17]{Shalev2007}).
    \item The norm $\norm{\,\cdot\,}_2 = d^{*v} (\,\cdot\,)$ is the dual norm of $\norm{\,\cdot\,}_2 = d^{v} (\,\cdot\,)$ (Hölder's inequality). 
    \item The local subgradient is upper bounded as $\norm{\vec g^v}_2 \leq R \max\{\sum^{|\vec\path|-1}_{k=k_{\vec\path} (v)} w_{(p_k, p_{k+1})}: \vec\path \in \pathSet\} = L^v_{\max}$. The maximum is achieved when $R$ requests need to be satisfied along the heaviest path from $v$ to a repository node.
    \item The Bregman divergence is upper bounded by $\frac{k}{2} (1- \frac{k}{N})=D^v_{\max}$ (see Eq.~\eqref{eq:qnorm_bregman_distance}).
    \item The $l_1$ norm is upper bounded by $\sqrt{N}\norm{\,\cdot\,}_2 = M^v d^v(\,\cdot\,)$ (Cauchy–Schwarz inequality).
\end{enumerate}

When $\Phi$ is the neg-entropy mirror map, assumption (A1)--(A2) in Sec.~\ref{sec:cn_regret_analysis} are satisfied as follows: 
\begin{enumerate}
    \item $\Phi$ is a mirror map (see Sec.~\ref{section:OMD}).
    \item  $\Phi$ is $\theta^v$-strongly convex w.r.t $\norm{\,\cdot\,}_1 = d^v({\,\cdot\,}) $, where $\frac{1}{k}$ (see \cite[Example 2.5]{ShalevOnlineLearning}).
    \item The norm $\norm{\,\cdot\,}_{\infty} = d^{*v} (\,\cdot\,)$ is the dual norm of $\norm{\,\cdot\,}_1 = d^{v} (\,\cdot\,)$ (Hölder's inequality). 
    \item The local subgradient is upper bounded as $\norm{\vec g^v}_\infty \leq R \max\{\sum^{|\vec\path|-1}_{k=k_{\vec\path} (v)} w_{(p_k, p_{k+1})}: \vec\path \in \pathSet\} = L^v_{\max}$. 
    \item The Bregman divergence is upper bounded by $k \log(N/k) = D^v_{\max}$ (see Eq.~\eqref{eq:qnorm_bregman_distance}).
    \item The $l_1$ norm is upper bounded by $1\norm{\,\cdot\,}_1 = M^v d^v(\,\cdot\,)$.
\end{enumerate}
\section{Supporting Lemma for the Proof of Theorem~\ref{theorem:cn_extended_fractional_regret}}
\begin{lemma}
When the local policy \LocalAlgoName{} in Algorithm~\ref{algo:cn_online_mirror_ascent} at every node $v \in \vertices$ is configured with the mirror map $\Phi^v$ (satisfying assumptions 1--5) and learning rate $\eta^v$, the update cost~\eqref{eq:cn_update_cost}  satisfies:
\begin{align}
     \underset{\{\vec{r}_1, \vec{r}_2, \dots, \vec{r}_t\} \in \mathcal{B}^T}{\sup} \left\{  \sum^T_{t=1} \sum_{v \in \vertices} \updatecost^v(\x^v_t, \x^v_{t+1})\right\} \leq \sum_{v \in \vertices }\frac{M^v w'^v_{\max} L^v_{\max} \eta^v}{\theta^v}  T.
\end{align}
\end{lemma}
\begin{proof}
% Let $w'^v_{\max} = \max\{w'^v_k: i \in \catalog \}$

Since $\updatecost^v(\x^v_{t}, \x^v_{t+1}) \leq w'^v_{\max} \norm{\x^v_{t+1} - \x^v_t}_1$ for every $v\in \vertices$, so the expected updated update can be bounded as follows
\begin{align}
    \sum^T_{k=1} \sum_{v \in \vertices} \updatecost^v(\x^v_{t}, \x^v_{t+1}) \leq \sum^T_{t=1} \sum_{v \in \vertices} w'^v_{\max} \norm{\x^v_{t+1} - \x^v_t}_1.
     \label{eq:cn_uc_bound}
\end{align}
We have from~\ref{asp:upperbound_norm}  $\norm{\x^v_{t+1} - \x^v_t}_1 \leq M^v d^v(\x^v_{t+1} - \x^v_t)$, then from Eq.~\eqref{eq:upper_bound_movement} we get
\begin{align}
    \norm{\x^v_{t+1} - \x^v_t}_1 \leq M^v d^v(\x^v_{t+1} - \x^v_t) \leq M^v \frac{L^v_{\max} \eta^v}{\theta^v}.
    \label{eq:cn_norm_bound}
\end{align}
Thus, using Eq.~\eqref{eq:cn_uc_bound} and Eq.~\eqref{eq:cn_norm_bound} the total update cost is given by 
\begin{align}
    \sum^T_{t=1} \sum_{v \in \vertices} \updatecost^v(\x^v_{t}, \x^v_{t+1}) \leq \sum_{v \in \vertices } \frac{M^v w'^v_{\max} L^v_{\max} \eta^v}{\theta^v}  T.
\end{align}
The above upper bound holds for any sequence of requests, so 
\begin{align}
     \underset{\{\vec{r}_1, \vec{r}_2, \dots, \vec{r}_t\} \in \mathcal{B}^T}{\sup} \left\{  \sum^T_{t=1} \sum_{v \in \vertices} \updatecost^v(\x^v_t, \x^v_{t+1})\right\} \leq  \sum_{v \in \vertices } \frac{M^v w'^v_{\max} L^v_{\max} \eta^v}{\theta^v}  T.
\end{align}


\end{proof}
\section{Proof of Theorem~\ref{theorem:cn_extended_fractional_regret}}
\label{proof:cn_extended_fractional_regret}
\begin{proof}
The extended regret~\eqref{eq:cn_fractional_extended_regret} can be bounded as 
\begin{align}
    &\widehat{\text{Regret}}_{T, \statesSetFrac}(\text{OMA}_{\Phi^{\vertices}}) \\
    &\leq \underset{\{\vec{r}_1, \vec{r}_2, \dots, \vec{r}_t\} \in \mathcal{B}^T}{\sup} \left\{ \sum^T_{t=1} G_{\vec r_t}(\x_*)- \sum^T_{t=1} G_{\vec{r}_t}(\x_t)  \right\} + \underset{\{\vec{r}_1, \vec{r}_2, \dots, \vec{r}_t\} \in \mathcal{B}^T}{\sup} \left\{  \sum^T_{t=1} \sum_{v \in \vertices} \updatecost^v(\x^v_t, \x^v_{t+1})\right\} \\
    &\leq   \text{Regret}_{T, \statesSetFrac}(\text{OMA}_{\Phi^{\vertices}})  + \underset{\{\vec{r}_1, \vec{r}_2, \dots, \vec{r}_t\} \in \mathcal{B}^T}{\sup} \left\{  \sum^T_{t=1} \sum_{v \in \vertices} \updatecost^v(\x^v_t, \x^v_{t+1})\right\} \\
    &\leq \sum_{v \in \vertices } \left(\frac{D^v_{\max}}{\eta^v} + \frac{\eta^v \left(L^v_{\max}\right)^2}{ 2 \theta^v} T \right) + \sum_{v \in \vertices } \frac{M^v w'^v_{\max} L^v_{\max} \eta^v}{\theta^v}  T.
\end{align}
By selecting the learning rate $\eta^v =\sqrt{\frac{2 D^v_{\max} \theta^v}{ \left( L^v_{\max} +2 M^v w'^v_{\max} / L^v_{\max} \right) L^v_{\max} T} }$ for every $v \in \vertices$ that gives the tightest upper bound, we finally get
\begin{align}
        \widehat{\text{Regret}}_{T, \statesSetFrac}(\text{OMA}_{\Phi^{\vertices}})  \leq  \left( \sum_{v \in \vertices} L^v_{\max}\sqrt{\frac{2D^v_{\max} \left( 1 + 2 M^v w'^v_{\max} / L^v_{\max} \right) }{\theta^v}}\right) \sqrt{T}.
\end{align}



\end{proof}



\section{Proof of Theorem~\ref{theorem:regret_generic_policy}}
\label{proof:regret_generic_policy}
\begin{proof}

When we restrict the maximization to the subset of integral allocations $\z\in\statesSetInt$, the optimal allocation $\z_* = {\arg\max}_{\z \in \statesSetInt} \sum^T_{t=1} G_{\vec r_t} (\z)$ can only lead to a lower gain, i.e.,
\begin{align}
   \sum^T_{t=1} G_{\vec r_t} (\z_*)
  \leq
 G_{\vec r_t} (\x_*),
  \label{eq:optimality_in_convx}
\end{align}
where $\x_* = \arg\max_{\x \in \mathcal{X}}\sum^T_{t=1} G_{\vec r_t} (\x)$ and $\z_* = \arg\max_{\z \in \mathcal{Z}}\sum^T_{t=1} G_{\vec r_t} (\z)$.


Take $\psi = 1 - \frac{1}{e}$ and a sequence of request batches $\{\vec r_t\}^T_{t=1}$, so we have the following

\begin{align}
   \psi \sum^T_{t=1} G_{\vec r_t} (\z_*) - \mathbb{E} \left[\sum^T_{t=1} G_{\vec r_t} (\z_t)\right]  &\stackrel{\eqref{eq:optimality_in_convx}} {\leq} \psi \sum^T_{t=1} G_{\vec r_t} (\x_*) - \mathbb{E} \left[\sum^T_{t=1} G_{\vec r_t} (\z_t)\right] 
   \stackrel{\eqref{eq:cn_lower_bound}}{\leq}\psi \sum^T_{t=1} G_{\vec r_t} (\x_*) - \psi \sum^T_{t=1} G_{\vec r_t} (\x_t)\\
    &= \psi \left( \sum^T_{t=1} G_{\vec r_t} (\x_*) -  \sum^T_{t=1} G_{\vec r_t} (\x_t)\right) .
\end{align}


By taking the supremum over all possible sequences of request batches we obtain 
\begin{align}
     \psi\text{-Regret}_T(\mathcal{A})  \leq \psi \cdot   \text{Regret}_{T, \statesSetFrac}(\mathcal{A}).
\end{align}
\end{proof}

\section{Proof of Theorem~\ref{theorem:cn_extended_psi_regret}}
\label{proof:cn_extended_psi_regret}
% movement_upperbound_l1
\begin{proof}
Similar the steps of the proof of Theorem~\ref{theorem:cn_extended_fractional_regret} in Appendix~\ref{proof:cn_extended_fractional_regret}, the extended $\psi$-regret~\eqref{eq:cn_psi_regret_extended} is bounded by
\begin{align}
\psi\text{-}\widehat{\text{Regret}}_{T, \statesSetInt}(\text{OMA}_{\Phi^{\vertices}}) \leq   \psi\text{-}{\text{Regret}}_{T, \statesSetInt}(\text{OMA}_{\Phi^{\vertices}})   + \underset{\{\vec{r}_1, \vec{r}_2, \dots, \vec{r}_t\} \in \mathcal{B}^T}{\sup} \left\{ \mathbb{E}\left[ \sum^T_{t=1} \sum_{v \in \vertices} \updatecost^v(\x^v_t, \x^v_{t+1})\right]\right\}. 
\label{eq:proof_extended_regret}
\end{align} 
Let $\vec w'^v = [w'^v_i]_{i \in \catalog}$ for every $v \in \vertices$, so we  have 
\begin{align}
  \mathbb{E}\left[  \sum^T_{t=1} \sum_{v \in \vertices} \updatecost^v(\x^v_t, \x^v_{t+1})\right] &\leq   \mathbb{E}\left[ \sum^T_{t=1} \sum_{v \in \vertices} \norm{\z^v_{t+1} - \z^v_t}_{1, \vec w'^v}\right]\\
  &\stackrel{\eqref{eq:movement_upperbound_l1}}{\leq}  k N \sum^T_{t=1} \sum_{v \in \vertices} w'^v_{\max} \norm{\z^v_{t+1} - \z^v_t}_{1}\\
  &\stackrel{\eqref{eq:cn_norm_bound}}{\leq} \sum_{v \in \vertices}k N  w'^v_{\max}\  M^v \frac{L^v_{\max} \eta^v}{\theta^v} T.
  \label{eq:proof_expected_update}
\end{align}
The above bound holds for any sequence of requests, so Eq.~\eqref{eq:proof_extended_regret}, Eq.~\eqref{eq:cn_raw_regret}, and Eq.~\eqref{eq:proof_expected_update} are combined to obtain 

\begin{align}
    \psi\text{-}\widehat{\text{Regret}}_{T, \statesSetInt}(\text{OMA}_{\Phi^{\vertices}}) \leq  \sum_{v \in \vertices}  \left(\frac{D^v_{\max}}{\eta^v} + \frac{\eta^v \left(L^v_{\max}\right)^2}{ 2 \theta^v} T \right) + \sum^T_{t=1} \sum_{v \in \vertices}   \frac{k N  M^vw'^v_{\max}L^v_{\max} \eta^v}{\theta^v}.
\end{align}
By selecting the learning rate $\eta^v = \sqrt{\frac{2 D^v_{\max} \theta^v}{ \left( L^v_{\max} +2 kNM^v w'^v_{\max} / L^v_{\max} \right) L^v_{\max} T} }$ for every $v\in\vertices$ that gives the tightest upper bound we finally obtain 
\begin{align}
      \widehat{\text{Regret}}_{T, \statesSetFrac}(\text{OMA}_{\Phi^{\vertices}})  \leq  \left( \sum_{v \in \vertices} L^v_{\max}\sqrt{\frac{2D^v_{\max} \left( 1 + 2 kN M^v w'^v_{\max} / L^v_{\max} \right) }{\theta^v}}\right) \sqrt{T}.
\end{align}

\end{proof}

\section{Proof of Corollary~\ref{corollary:cn_integral_offline_problem}}
\label{proof:cn_integral_offline_problem}
\begin{proof}
Consider the following
\begin{align}
    \mathbb{E} \left[ G_T(\bar \z) \right] \stackrel{\eqref{eq:cn_lower_bound}}{\geq} \psi  G_T(\bar \x) \stackrel{\eqref{eq:cn_static_ineq}}{\geq} \psi\left(  G_T(\x_*)  - \left(\sum_{v \in \vertices} L^v_{\max} \sqrt{\frac{2 D^v_{\max}}{\theta^v} }\right) \frac{1}{\sqrt{K}}\right).
    \end{align}
This concludes the proof.
\end{proof}
